# Supplementary material for: FEASTS Compared with Simulations: Abnormally Irregular and Extended HI Morphologies at a Column Density of $10^{18}\,\text{cm}^{-2}$ in TNG50 and Auriga
Source: arXiv:2512.07223 ancillary file (2025-12-08)

# NGC 7331

$I_{18} = 0.10$   
 $\log(S_{18}/S_{19}) = 0.22$   
 $\log(S_{19}/S_{20}) = 0.30$

$\log(M_*/M_\odot) = 11.00$   
 $\log(M_{\text{H I}}/M_\odot) = 10.10$   
 $i = 76^\circ$

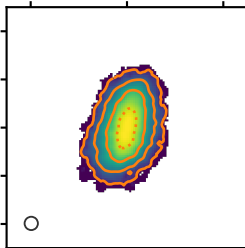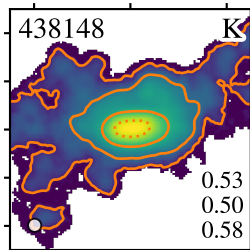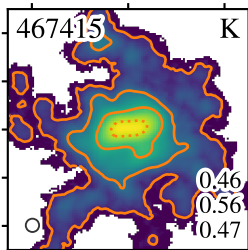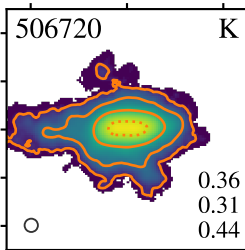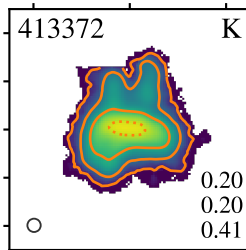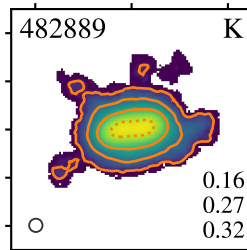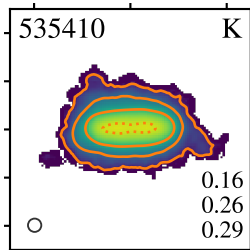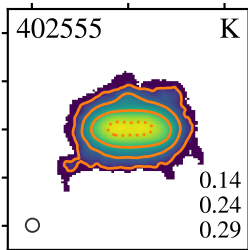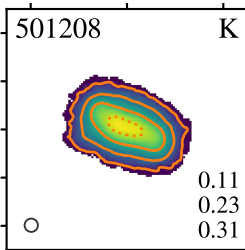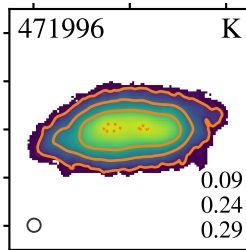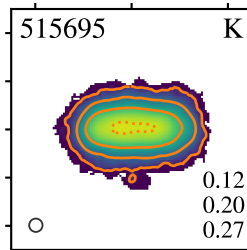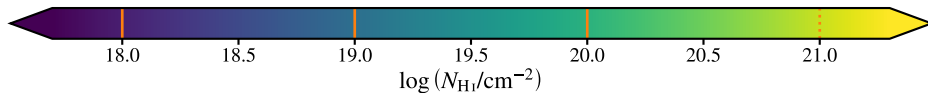

# NGC 2841

$I_{18} = 0.15$   
 $\log(S_{18}/S_{19}) = 0.18$   
 $\log(S_{19}/S_{20}) = 0.32$

$\log(M_*/M_\odot) = 10.93$   
 $\log(M_{\text{H I}}/M_\odot) = 9.99$   
 $i = 63^\circ$

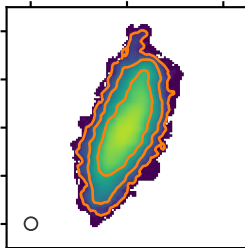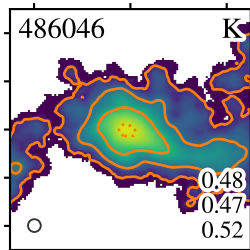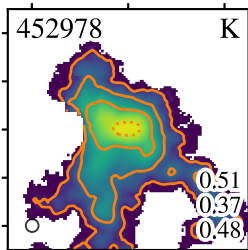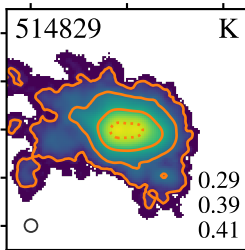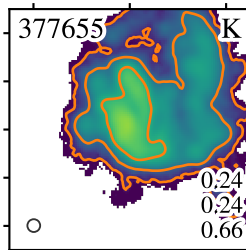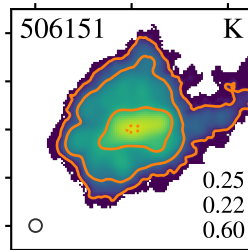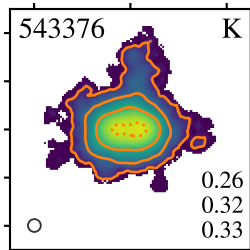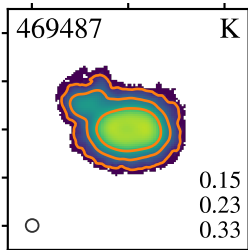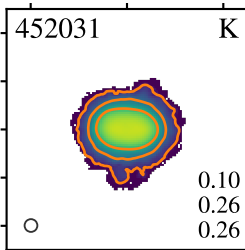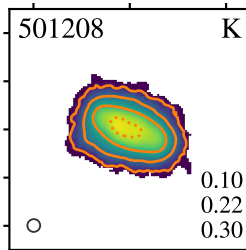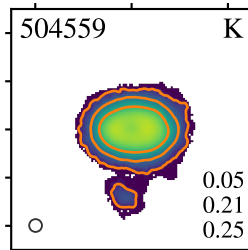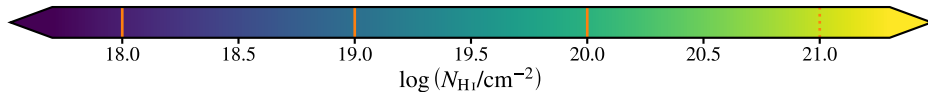

# NGC 4565

$I_{18} = 0.19$   
 $\log(S_{18}/S_{19}) = 0.25$   
 $\log(S_{19}/S_{20}) = 0.28$

$\log(M_*/M_\odot) = 10.88$   
 $\log(M_{\text{H I}}/M_\odot) = 9.99$   
 $i = 80^\circ$

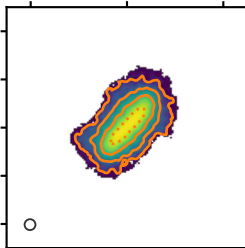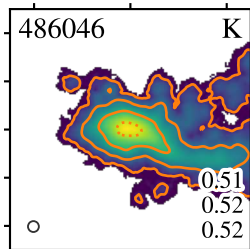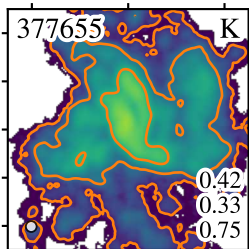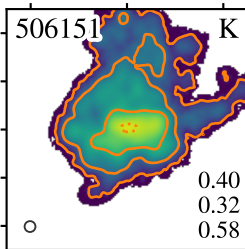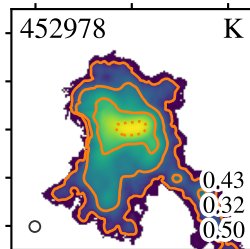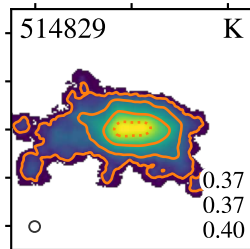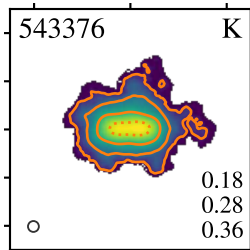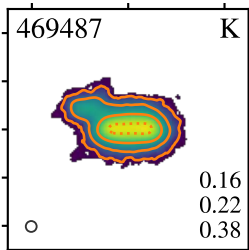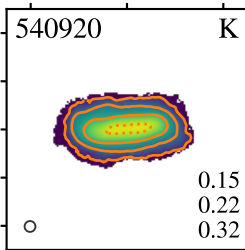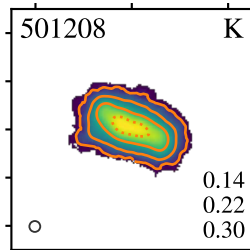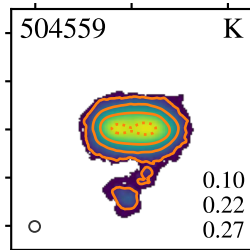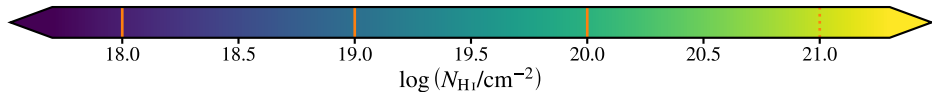

# NGC 5907

$I_{18} = 0.16$   
 $\log(S_{18}/S_{19}) = 0.19$   
 $\log(S_{19}/S_{20}) = 0.32$

$\log(M_*/M_\odot) = 10.84$   
 $\log(M_{\text{H I}}/M_\odot) = 10.37$   
 $i = 84^\circ$

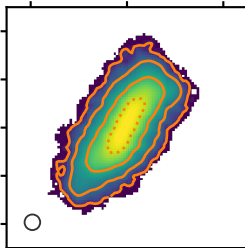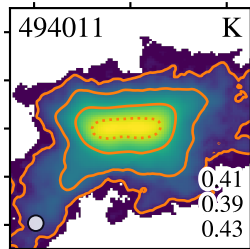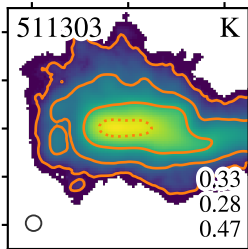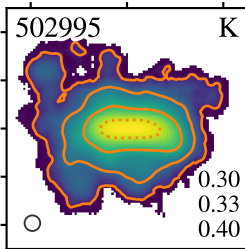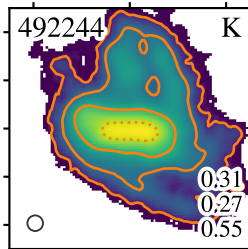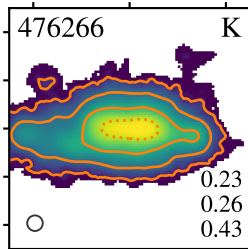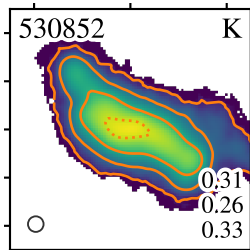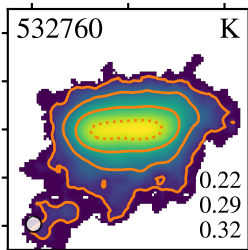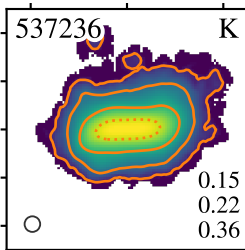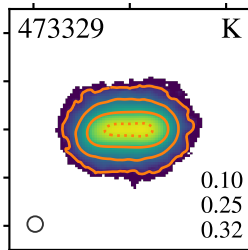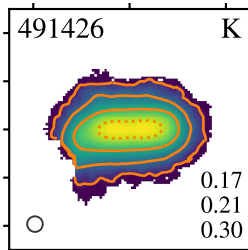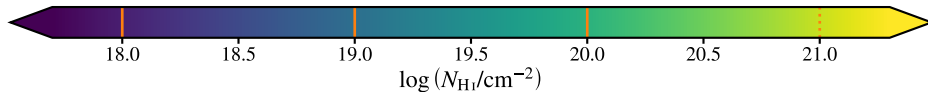

# NGC 3521

$I_{18} = 0.24$   
 $\log(S_{18}/S_{19}) = 0.27$   
 $\log(S_{19}/S_{20}) = 0.31$

$\log(M_*/M_\odot) = 10.83$   
 $\log(M_{\text{H I}}/M_\odot) = 9.99$   
 $i = 63^\circ$

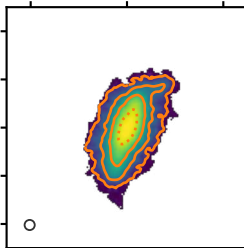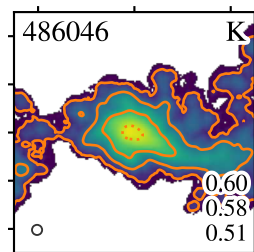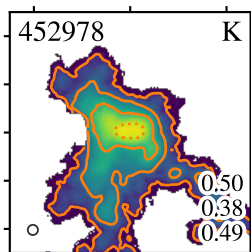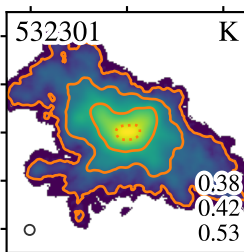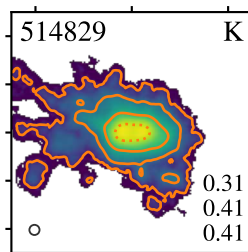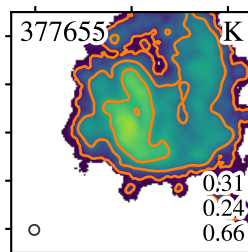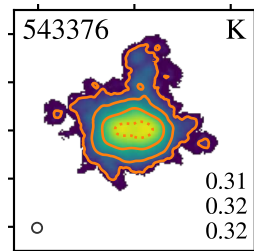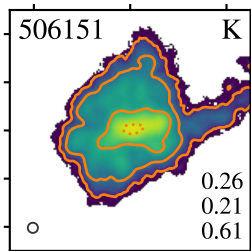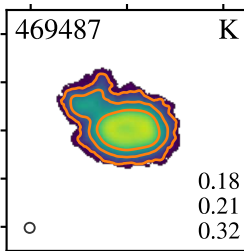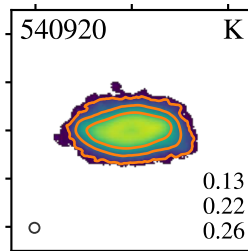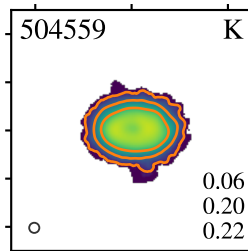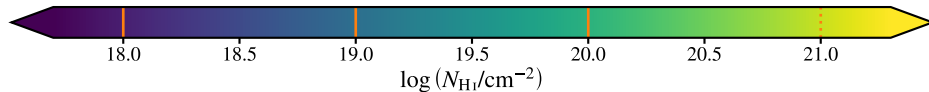

# NGC 4725

$I_{18} = 0.13$   
 $\log(S_{18}/S_{19}) = 0.25$   
 $\log(S_{19}/S_{20}) = 0.32$

$\log(M_*/M_\odot) = 10.76$   
 $\log(M_{\text{H I}}/M_\odot) = 9.68$   
 $i = 47^\circ$

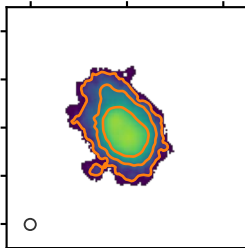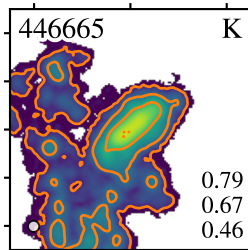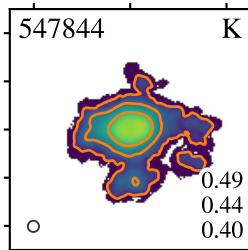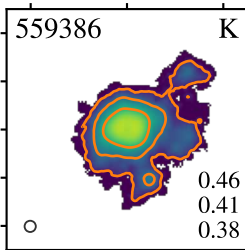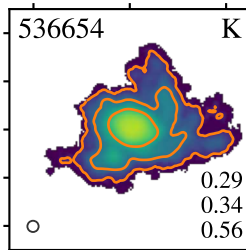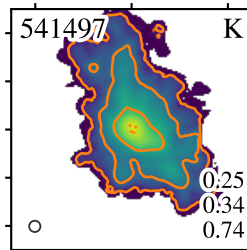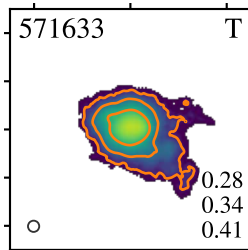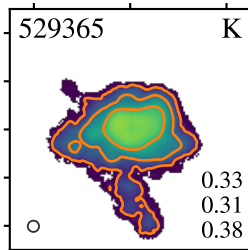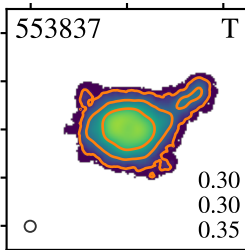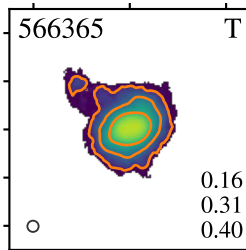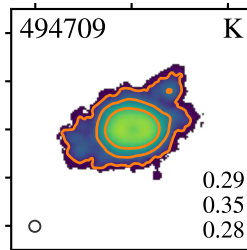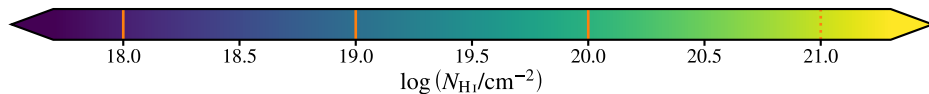

# NGC 6384

$I_{18} = 0.12$   
 $\log(S_{18}/S_{19}) = 0.24$   
 $\log(S_{19}/S_{20}) = 0.30$

$\log(M_*/M_\odot) = 10.76$   
 $\log(M_{\text{H I}}/M_\odot) = 10.16$   
 $i = 60^\circ$

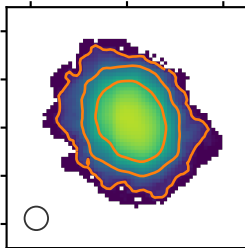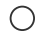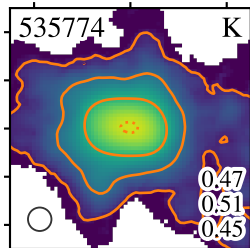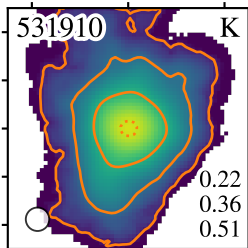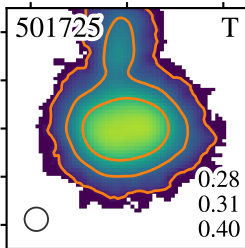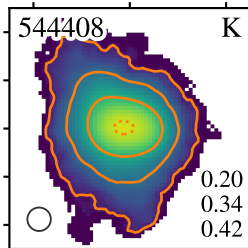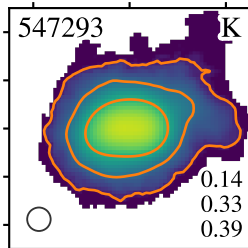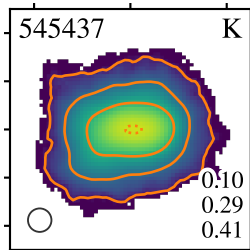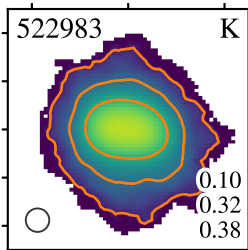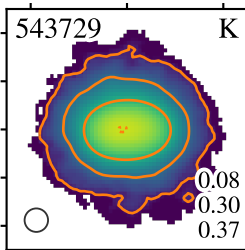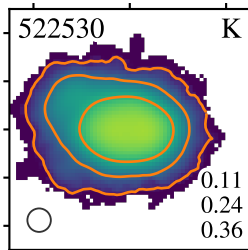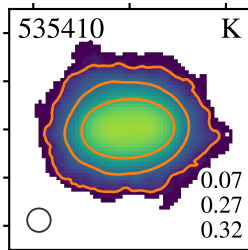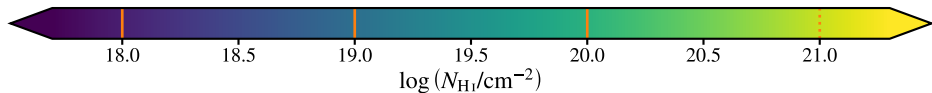

# NGC 5194

$I_{18} = 0.16$   
 $\log(S_{18}/S_{19}) = 0.25$   
 $\log(S_{19}/S_{20}) = 0.74$

$\log(M_*/M_\odot) = 10.73$   
 $\log(M_{\text{H I}}/M_\odot) = 9.72$   
 $i = 33^\circ$

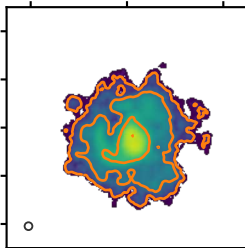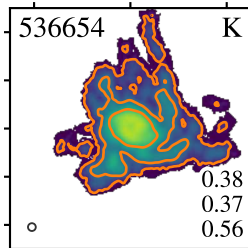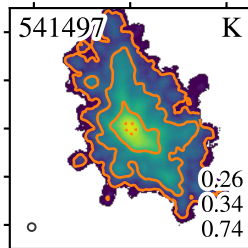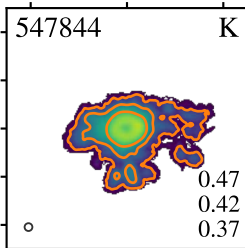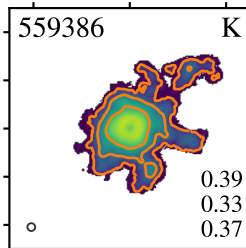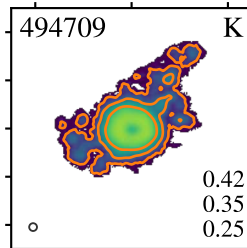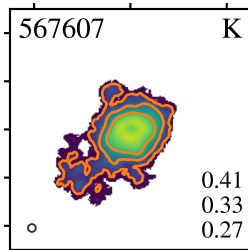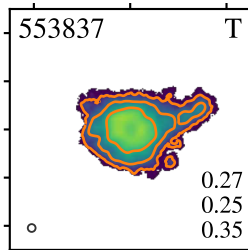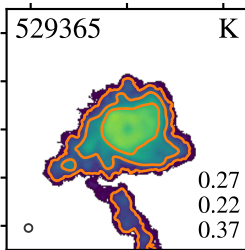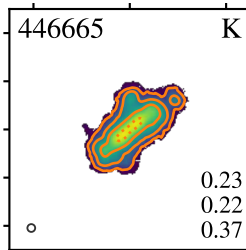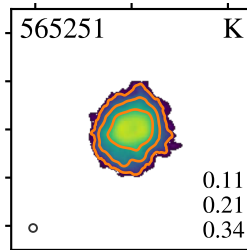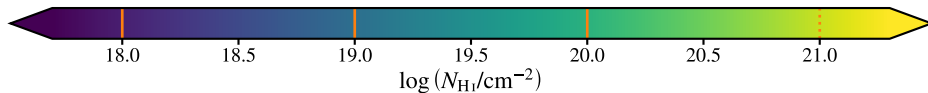

# NGC 5055

$I_{18} = 0.09$   
 $\log(S_{18}/S_{19}) = 0.14$   
 $\log(S_{19}/S_{20}) = 0.29$

$\log(M_*/M_\odot) = 10.72$   
 $\log(M_{\text{H I}}/M_\odot) = 10.03$   
 $i = 56^\circ$

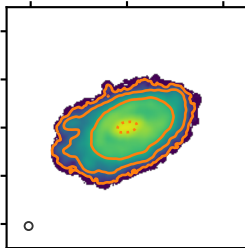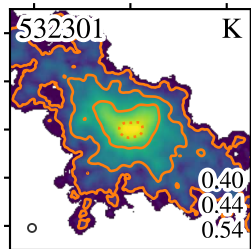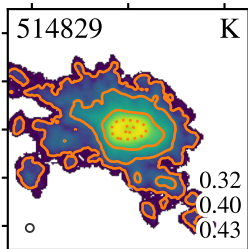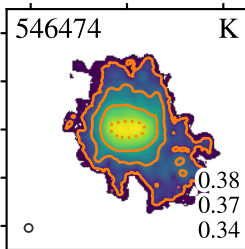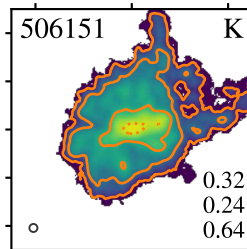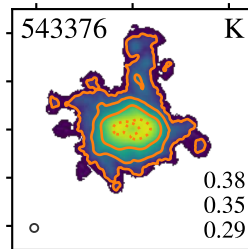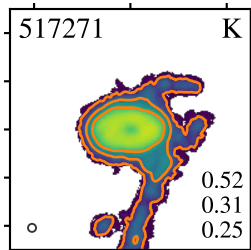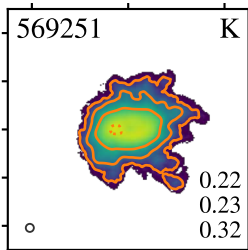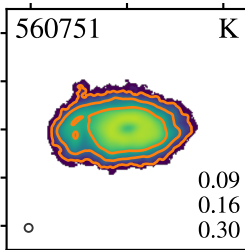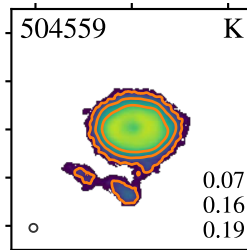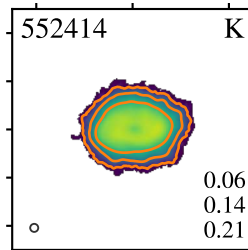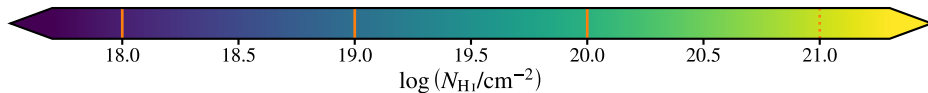

# NGC 891

$I_{18} = 0.16$   
 $\log(S_{18}/S_{19}) = 0.24$   
 $\log(S_{19}/S_{20}) = 0.35$

$\log(M_*/M_\odot) = 10.72$   
 $\log(M_{\text{H I}}/M_\odot) = 9.69$   
 $i = 90^\circ$

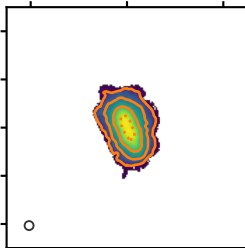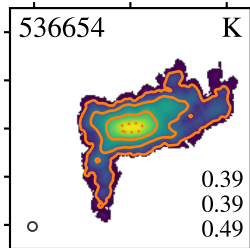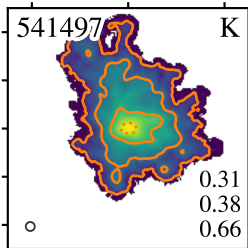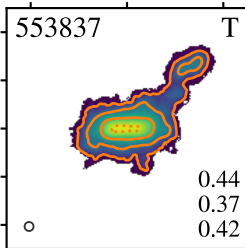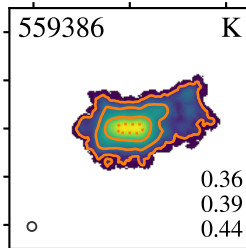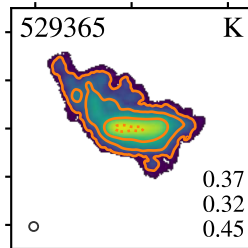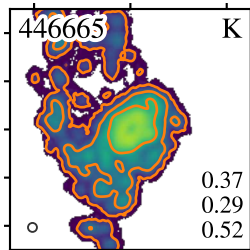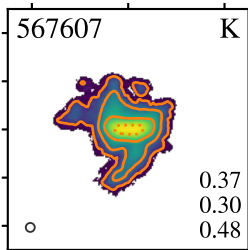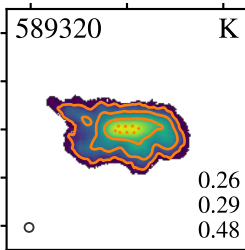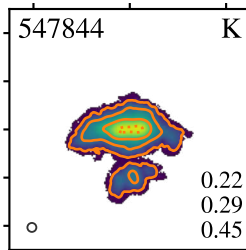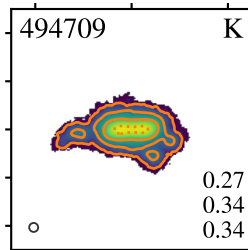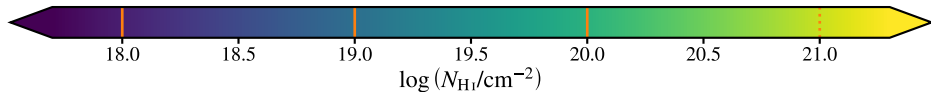

# NGC 4303

$I_{18} = 0.23$   
 $\log(S_{18}/S_{19}) = 0.39$   
 $\log(S_{19}/S_{20}) = 0.39$

$\log(M_*/M_\odot) = 10.67$   
 $\log(M_{\text{H I}}/M_\odot) = 9.88$   
 $i = 27^\circ$

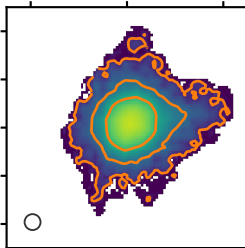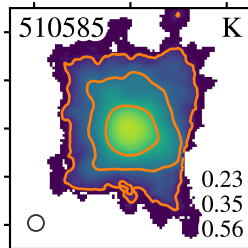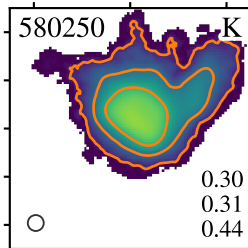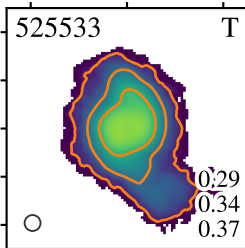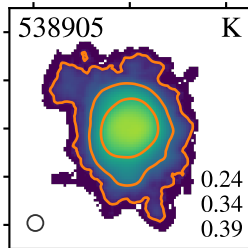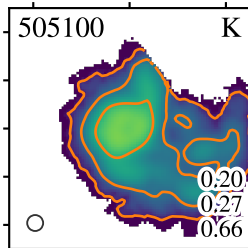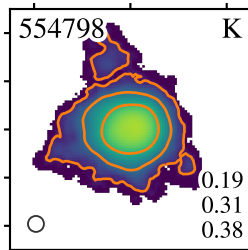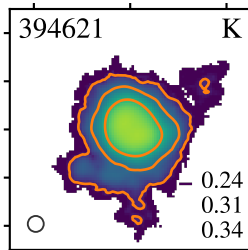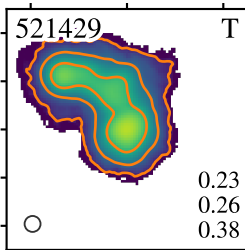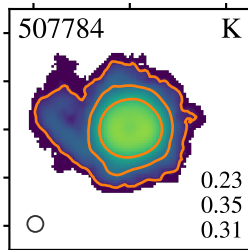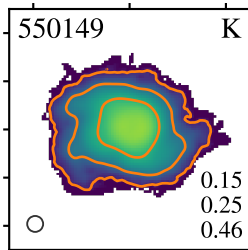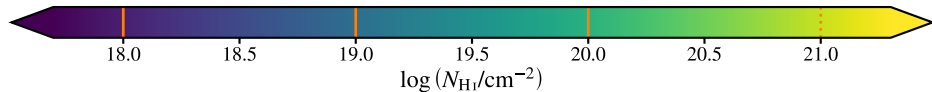

# NGC 4258

$$I_{18} = 0.23$$

$$\log(S_{18}/S_{19}) = 0.22$$

$$\log(S_{19}/S_{20}) = 0.25$$

$$\log(M_*/M_\odot) = 10.67$$

$$\log(M_{\text{H I}}/M_\odot) = 9.83$$

$$i = 75^\circ$$

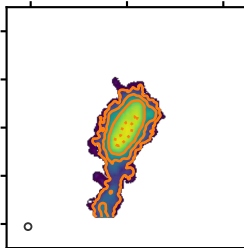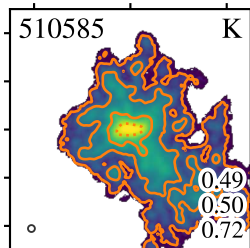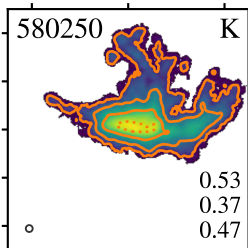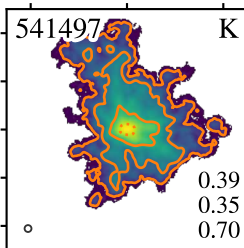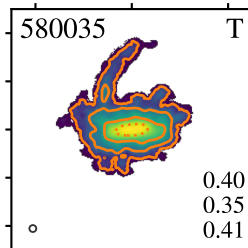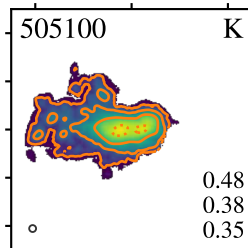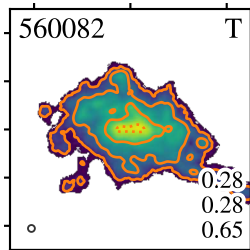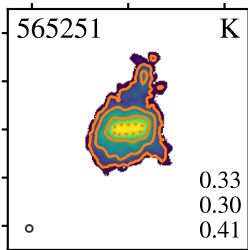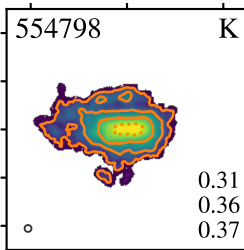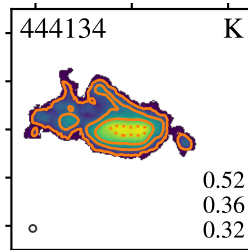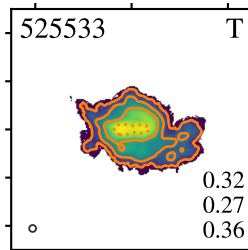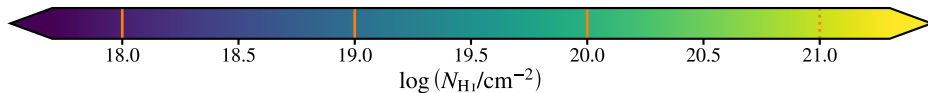

# NGC 4527

$$I_{18} = 0.23$$

$$\log(S_{18}/S_{19}) = 0.31$$

$$\log(S_{19}/S_{20}) = 0.45$$

$$\log(M_*/M_\odot) = 10.66$$

$$\log(M_{\text{H I}}/M_\odot) = 9.94$$

$$i = 74^\circ$$

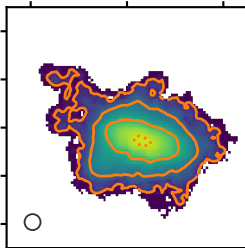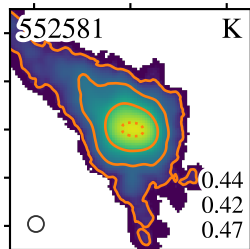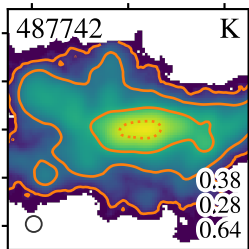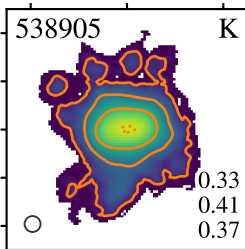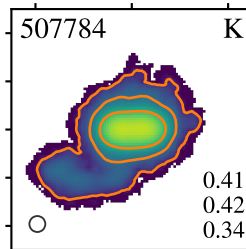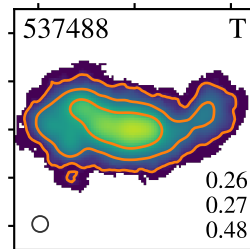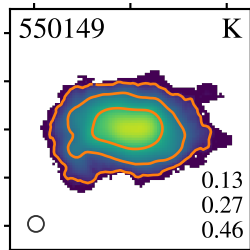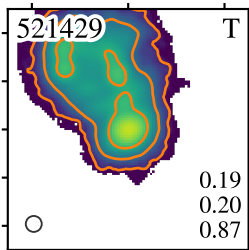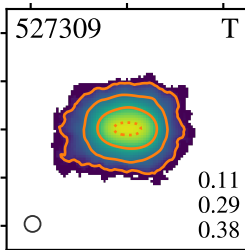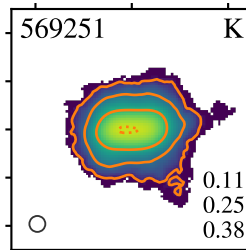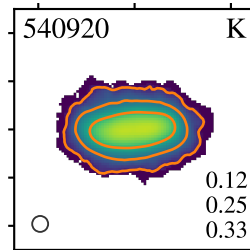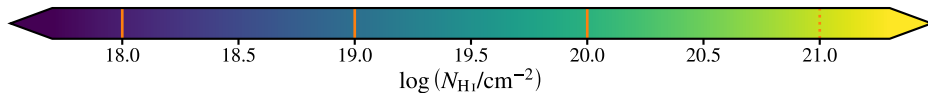

# NGC 4414

$I_{18} = 0.13$   
 $\log(S_{18}/S_{19}) = 0.25$   
 $\log(S_{19}/S_{20}) = 0.48$

$\log(M_*/M_\odot) = 10.65$   
 $\log(M_{\text{H I}}/M_\odot) = 9.73$   
 $i = 57^\circ$

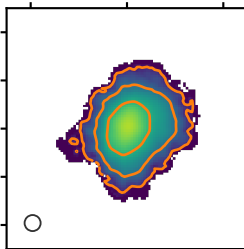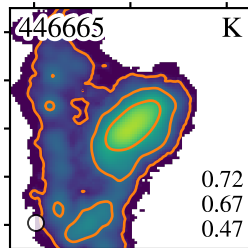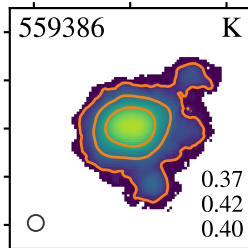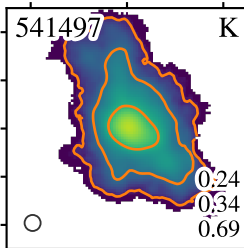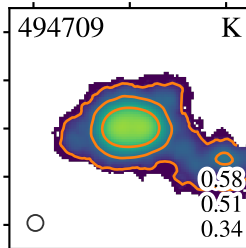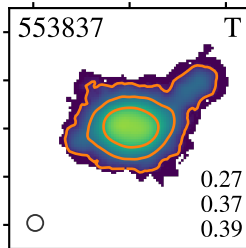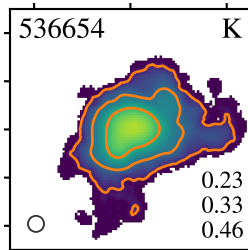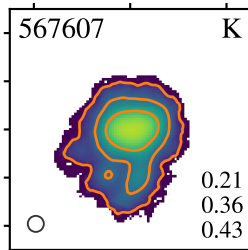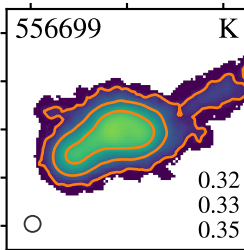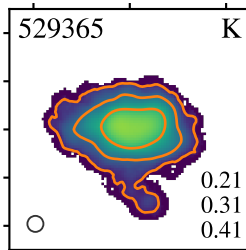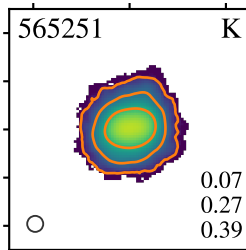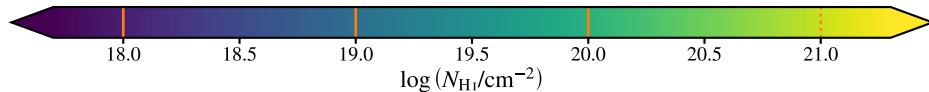

# NGC 3718

$I_{18} = 0.22$   
 $\log(S_{18}/S_{19}) = 0.22$   
 $\log(S_{19}/S_{20}) = 0.43$

$\log(M_*/M_\odot) = 10.48$   
 $\log(M_{\text{H I}}/M_\odot) = 10.02$   
 $i = 67^\circ$

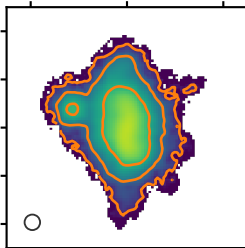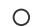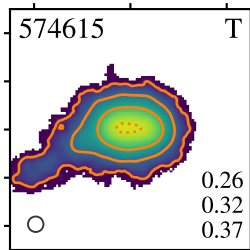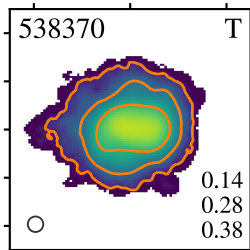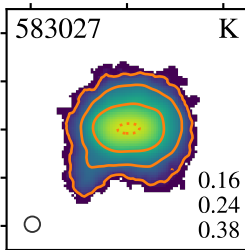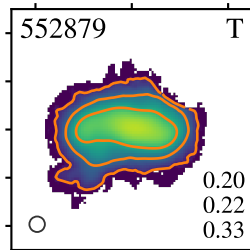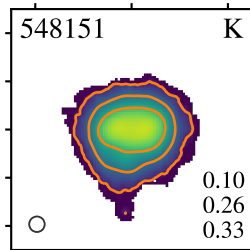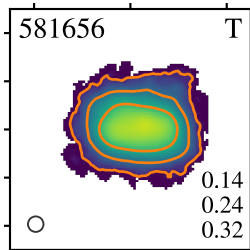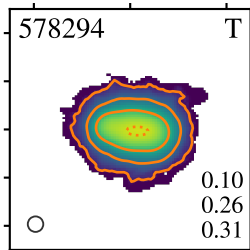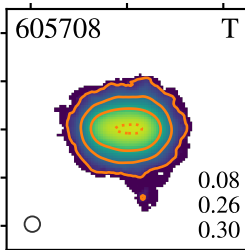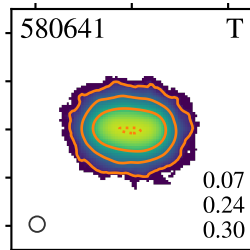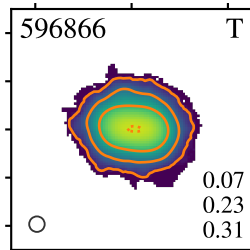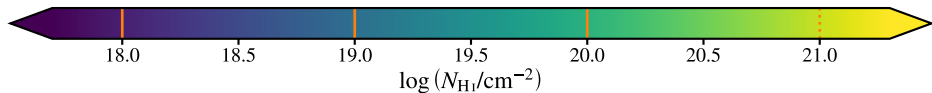

NGC 5775

$I_{18} = 0.15$   
 $\log(S_{18}/S_{19}) = 0.27$   
 $\log(S_{19}/S_{20}) = 0.33$

$\log(M_*/M_\odot) = 10.47$   
 $\log(M_{\text{H I}}/M_\odot) = 10.05$   
 $i = 82^\circ$

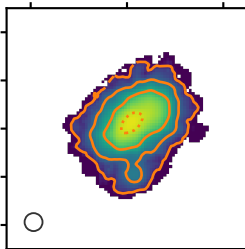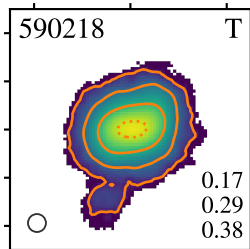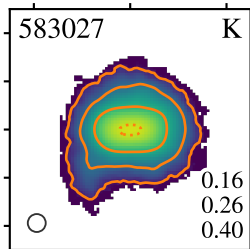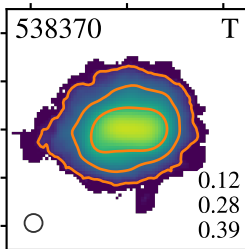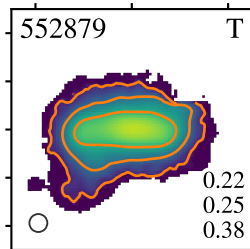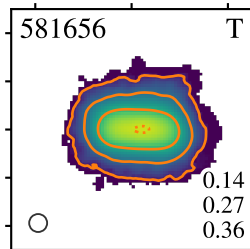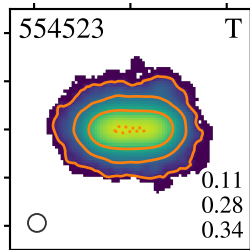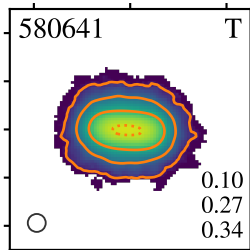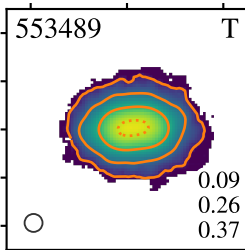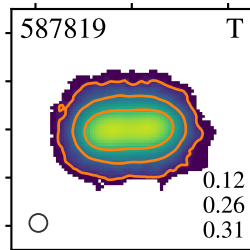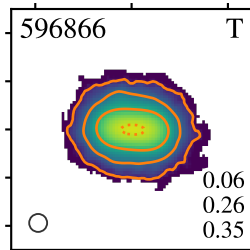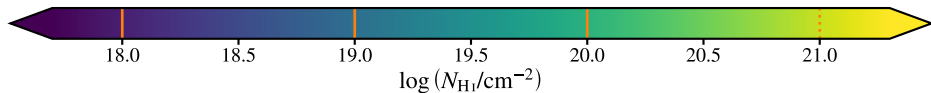

# NGC 2903

$I_{18} = 0.16$   
 $\log(S_{18}/S_{19}) = 0.23$   
 $\log(S_{19}/S_{20}) = 0.31$

$\log(M_*/M_\odot) = 10.42$   
 $\log(M_{\text{H I}}/M_\odot) = 9.63$   
 $i = 61^\circ$

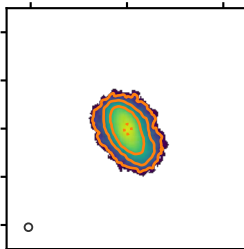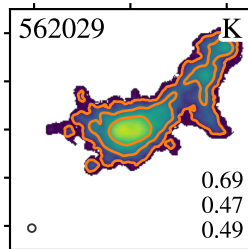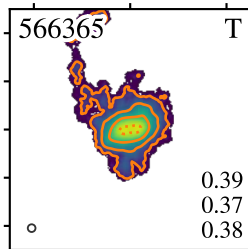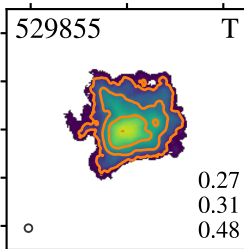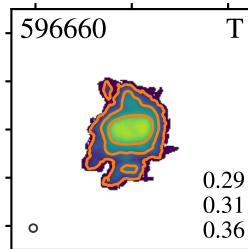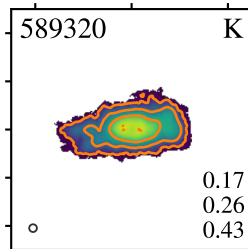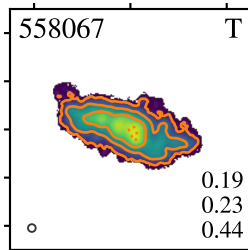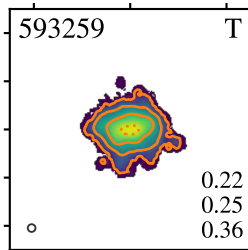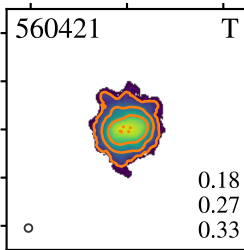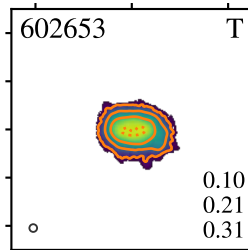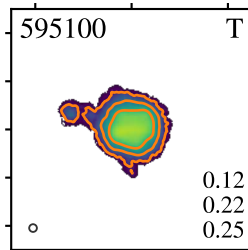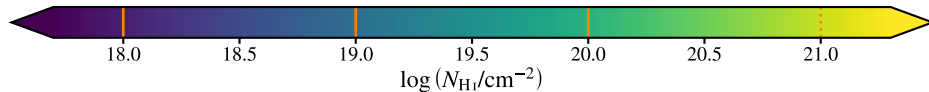

# NGC 5457

$I_{18} = 0.11$   
 $\log(S_{18}/S_{19}) = 0.12$   
 $\log(S_{19}/S_{20}) = 0.25$

$\log(M_*/M_\odot) = 10.39$   
 $\log(M_{\text{H I}}/M_\odot) = 10.35$   
 $i = 22^\circ$

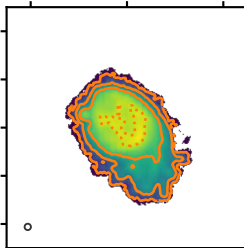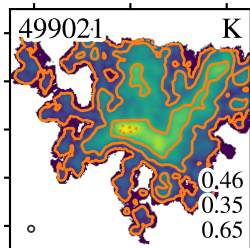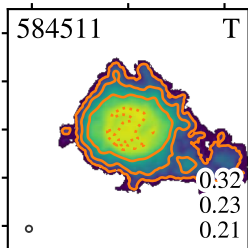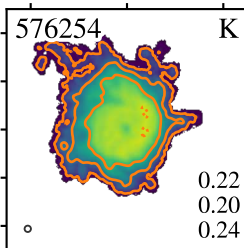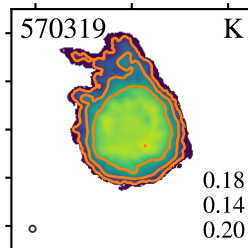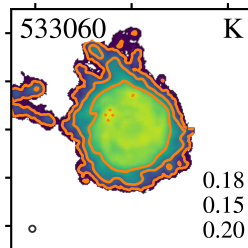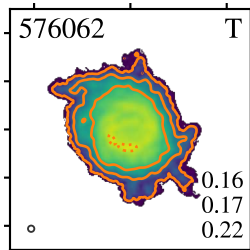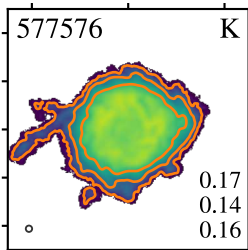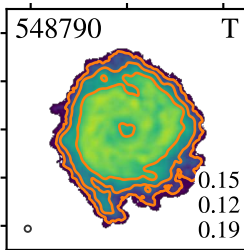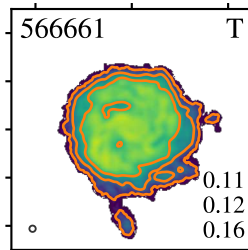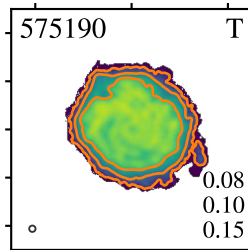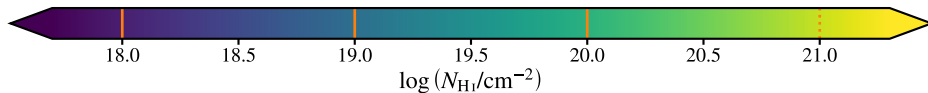

# NGC 3344

$I_{18} = 0.10$   
 $\log(S_{18}/S_{19}) = 0.20$   
 $\log(S_{19}/S_{20}) = 0.49$

$\log(M_*/M_\odot) = 10.29$   
 $\log(M_{\text{H I}}/M_\odot) = 9.72$   
 $i = 27^\circ$

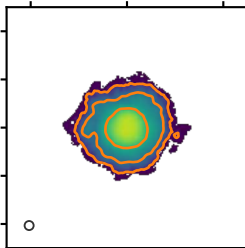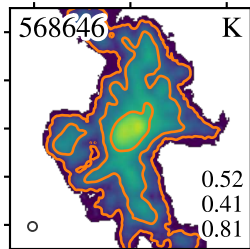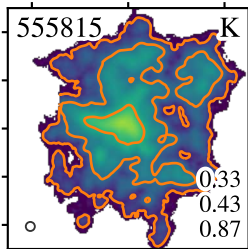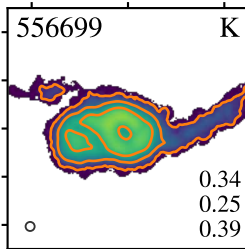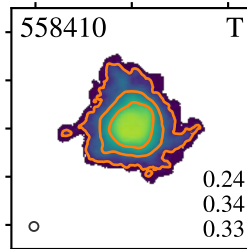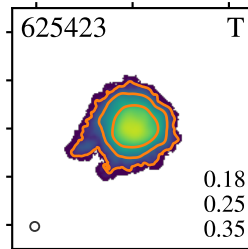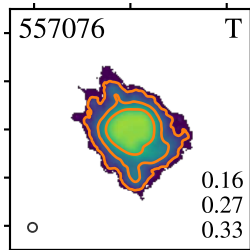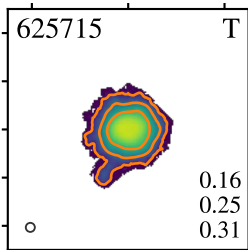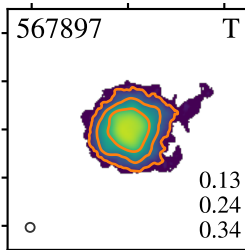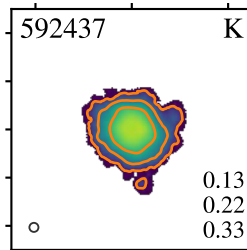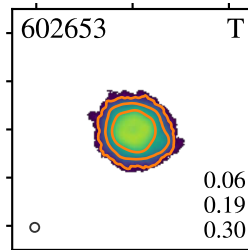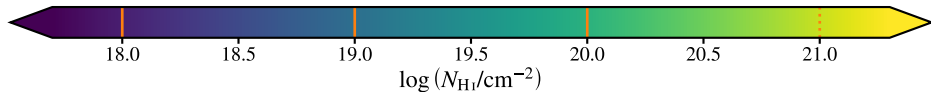

# NGC 628

$I_{18} = 0.07$   
 $\log(S_{18}/S_{19}) = 0.17$   
 $\log(S_{19}/S_{20}) = 0.27$

$\log(M_*/M_\odot) = 10.24$   
 $\log(M_{\text{H I}}/M_\odot) = 10.08$   
 $i = 31^\circ$

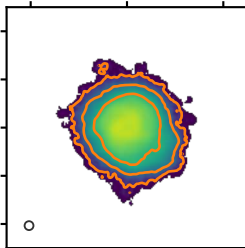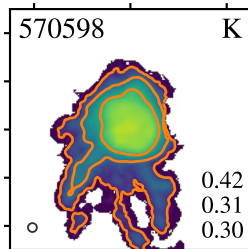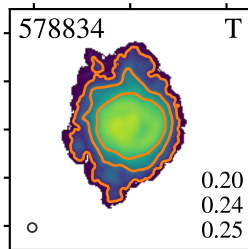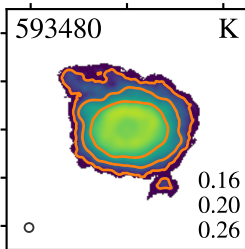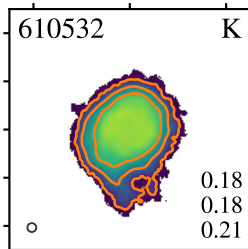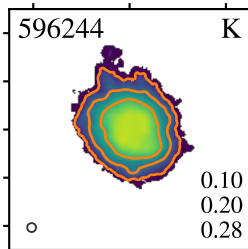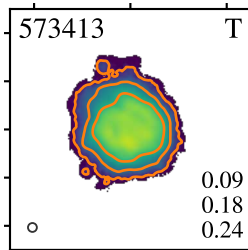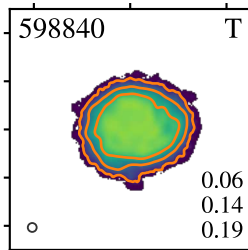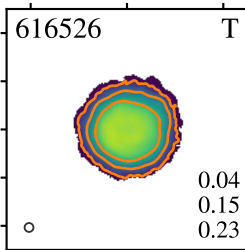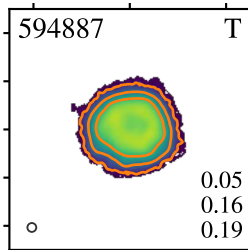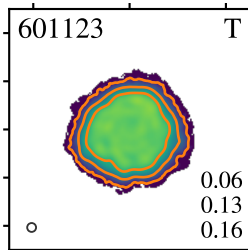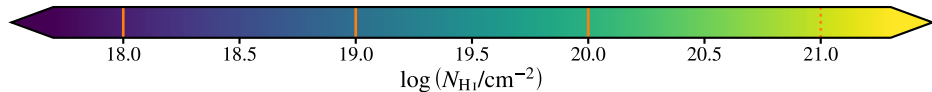

# NGC 4517

$I_{18} = 0.17$   
 $\log(S_{18}/S_{19}) = 0.27$   
 $\log(S_{19}/S_{20}) = 0.35$

$\log(M_*/M_\odot) = 10.22$   
 $\log(M_{\text{H I}}/M_\odot) = 9.63$   
 $i = 83^\circ$

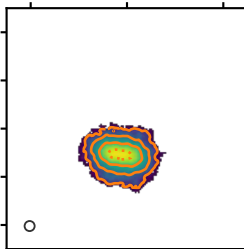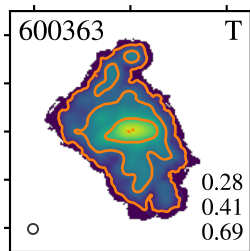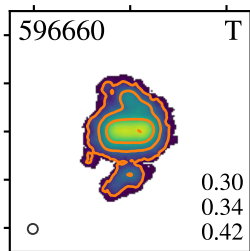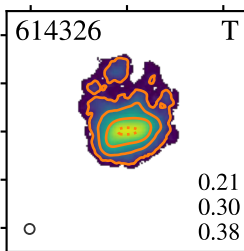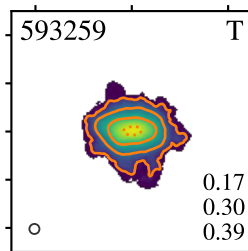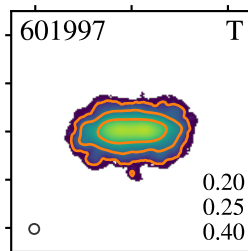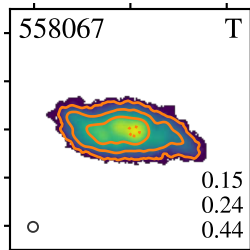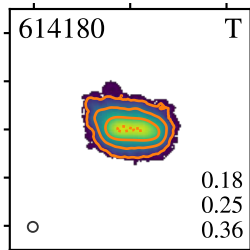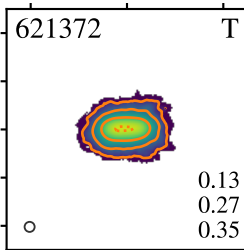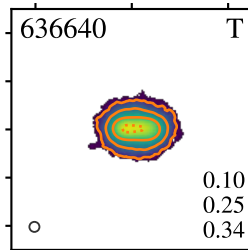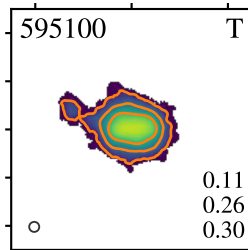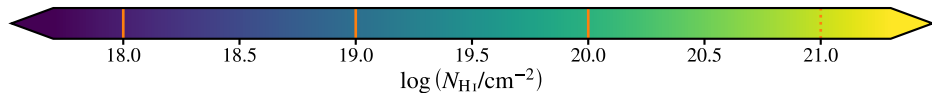

NGC 3338

$$I_{18} = 0.18$$

$$\log(S_{18}/S_{19}) = 0.26$$

$$\log(S_{19}/S_{20}) = 0.41$$

$$\log(M_*/M_\odot) = 10.20$$

$$\log(M_{\text{H I}}/M_\odot) = 10.14$$

$$i = 61^\circ$$

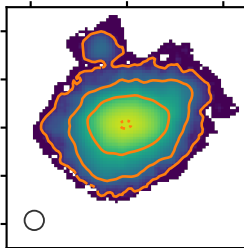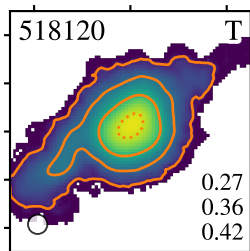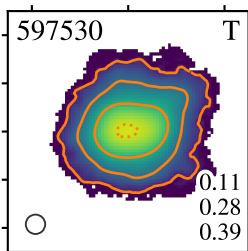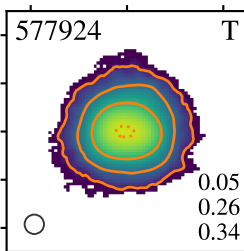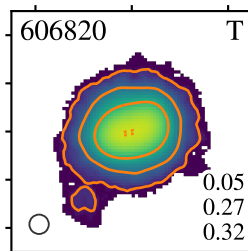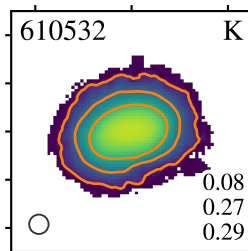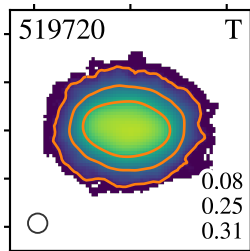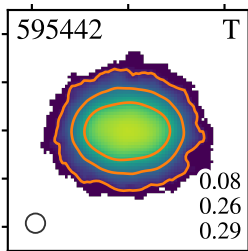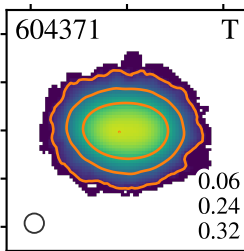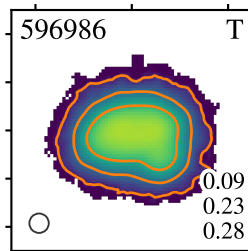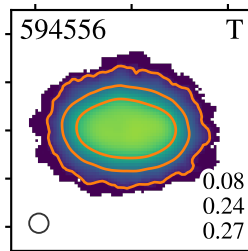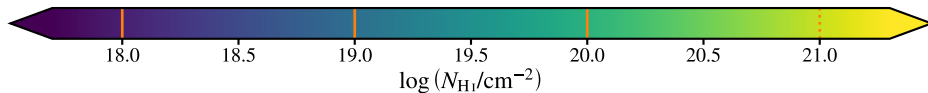

# NGC 5248

$I_{18} = 0.14$   
 $\log(S_{18}/S_{19}) = 0.32$   
 $\log(S_{19}/S_{20}) = 0.34$

$\log(M_*/M_\odot) = 10.20$   
 $\log(M_{\text{H I}}/M_\odot) = 9.54$   
 $i = 39^\circ$

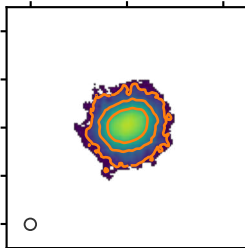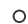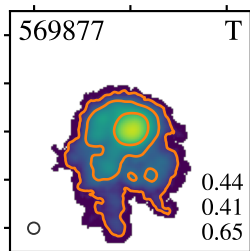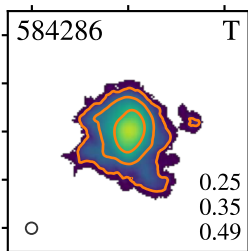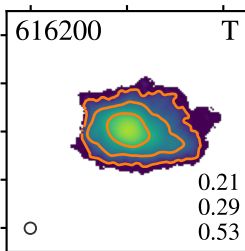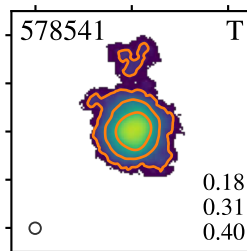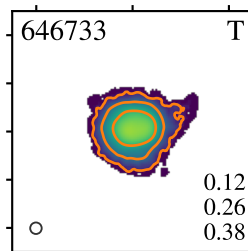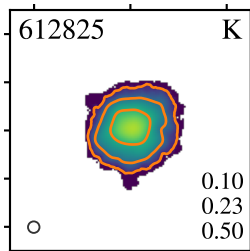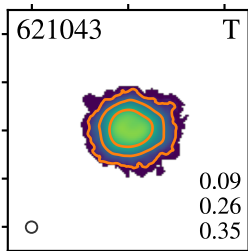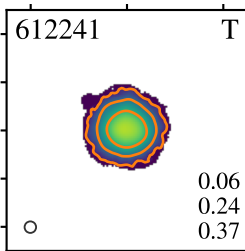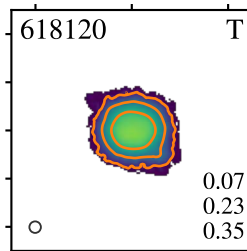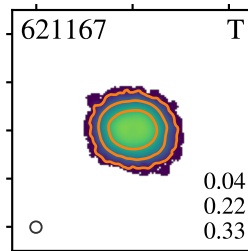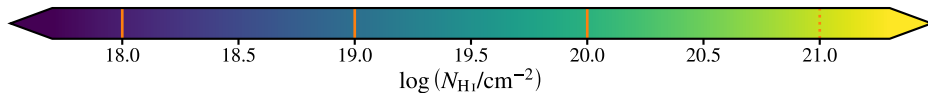

# NGC 3198

$I_{18} = 0.16$   
 $\log(S_{18}/S_{19}) = 0.21$   
 $\log(S_{19}/S_{20}) = 0.27$

$\log(M_*/M_\odot) = 10.05$   
 $\log(M_{\text{H I}}/M_\odot) = 10.05$   
 $i = 70^\circ$

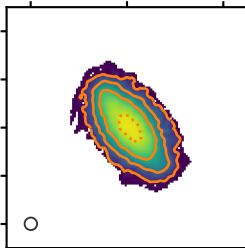

○

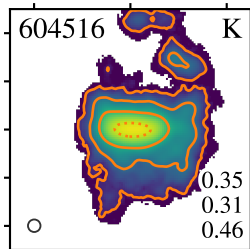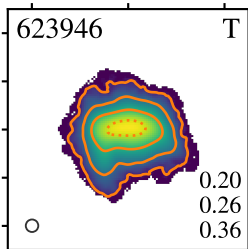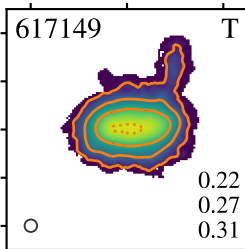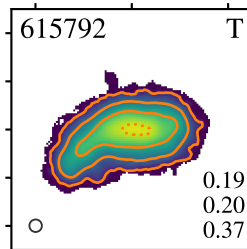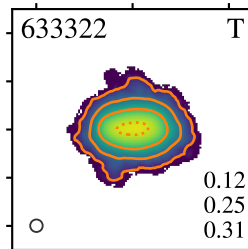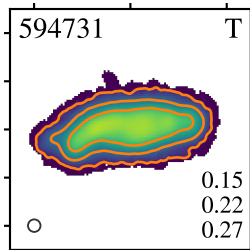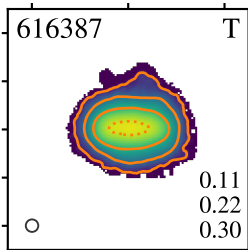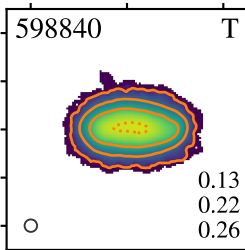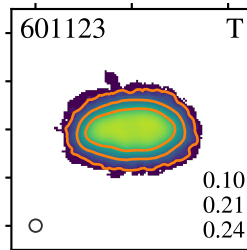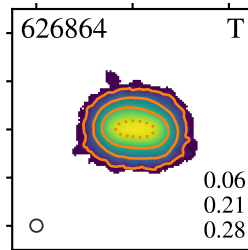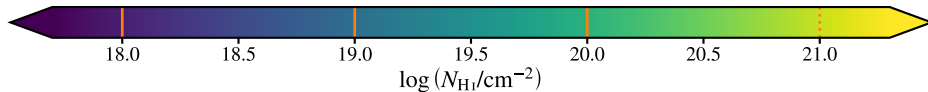

# NGC 4631

$I_{18} = 0.16$   
 $\log(S_{18}/S_{19}) = 0.13$   
 $\log(S_{19}/S_{20}) = 0.50$

$\log(M_*/M_\odot) = 10.05$   
 $\log(M_{\text{H I}}/M_\odot) = 10.01$   
 $i = 77^\circ$

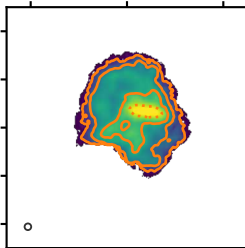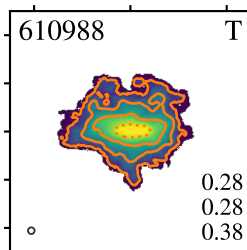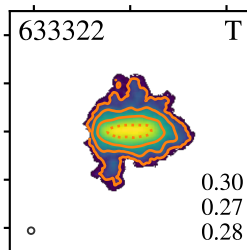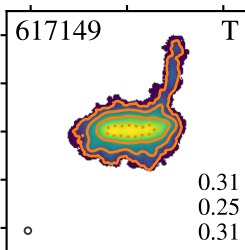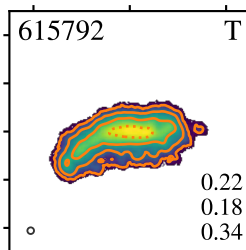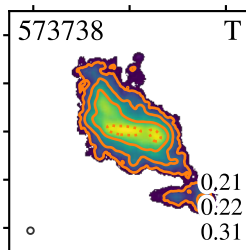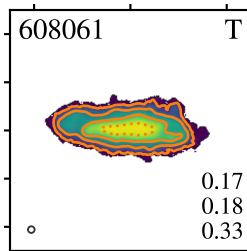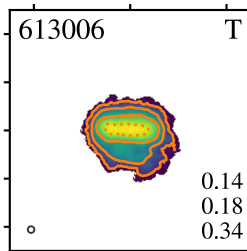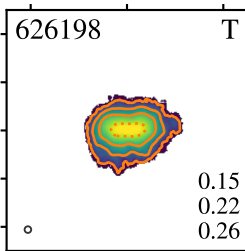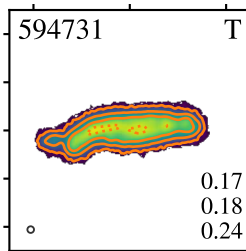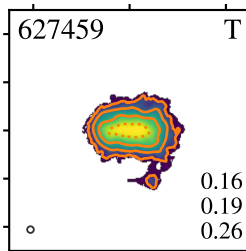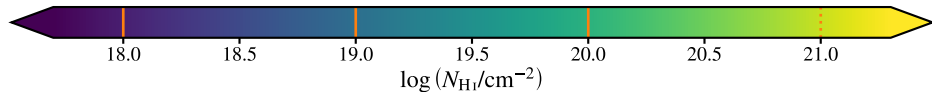

# NGC 3486

$I_{18} = 0.14$   
 $\log(S_{18}/S_{19}) = 0.27$   
 $\log(S_{19}/S_{20}) = 0.36$

$\log(M_*/M_\odot) = 10.00$   
 $\log(M_{\text{H I}}/M_\odot) = 9.85$   
 $i = 42^\circ$

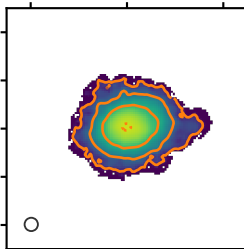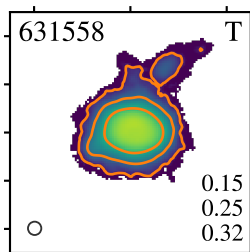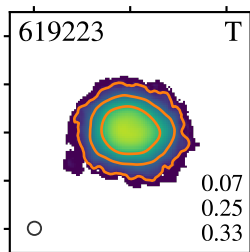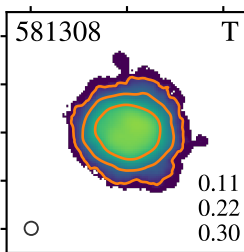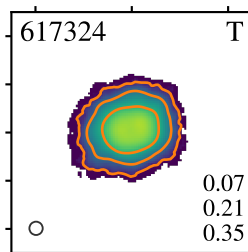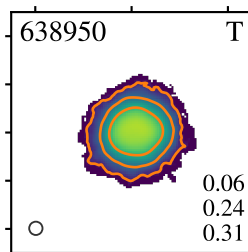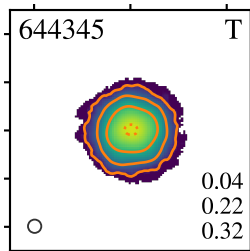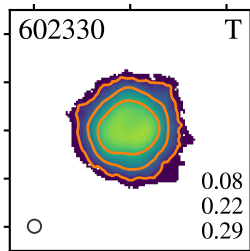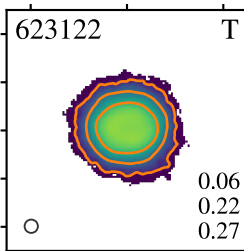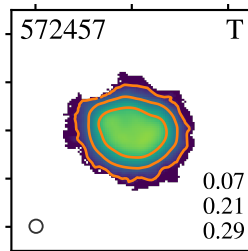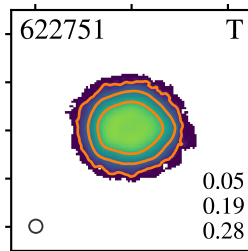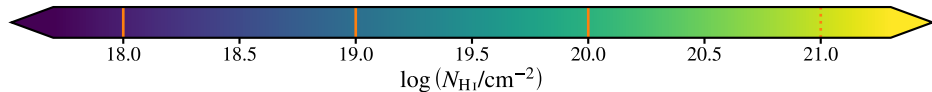

# NGC 3556

$$I_{18} = 0.17$$

$$\log(S_{18}/S_{19}) = 0.24$$

$$\log(S_{19}/S_{20}) = 0.37$$

$$\log(M_*/M_\odot) = 9.94$$

$$\log(M_{\text{H I}}/M_\odot) = 9.59$$

$$i = 73^\circ$$

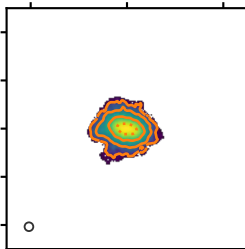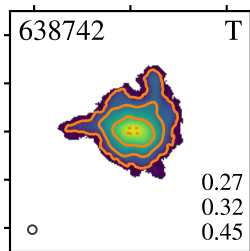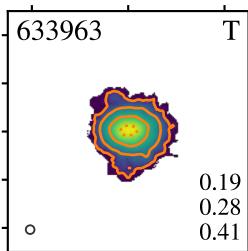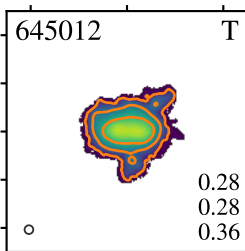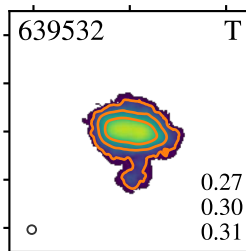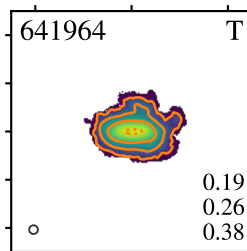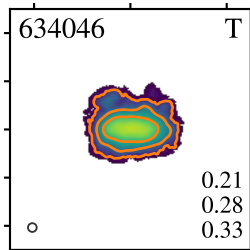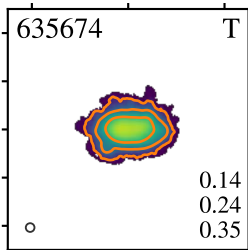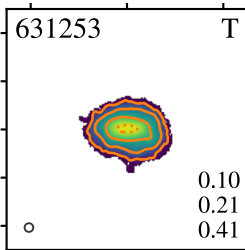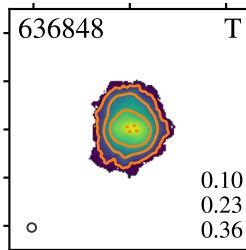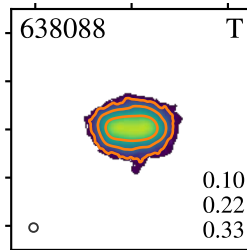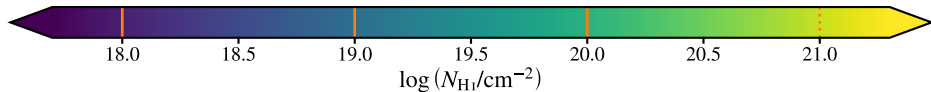

# NGC 4559

$I_{18} = 0.12$   
 $\log(S_{18}/S_{19}) = 0.29$   
 $\log(S_{19}/S_{20}) = 0.27$

$\log(M_*/M_\odot) = 9.81$   
 $\log(M_{\text{H I}}/M_\odot) = 9.80$   
 $i = 63^\circ$

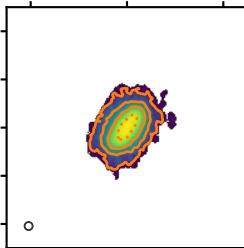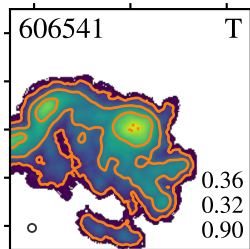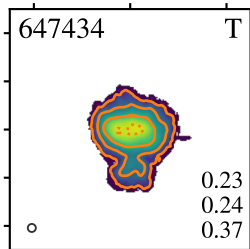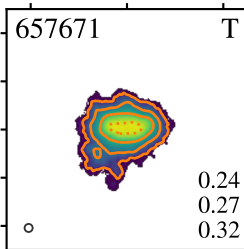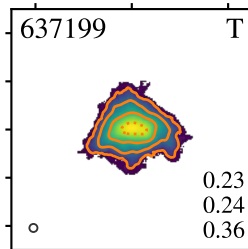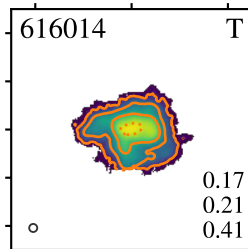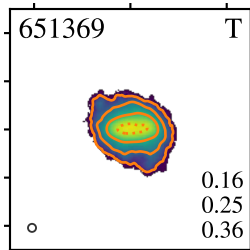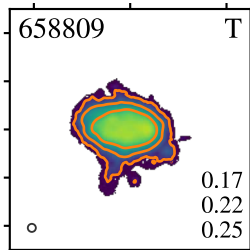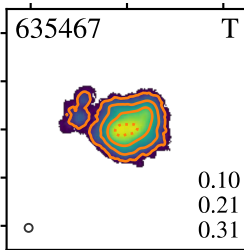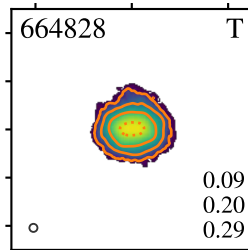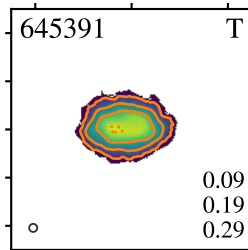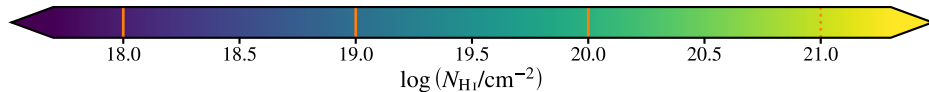

# NGC 864

$I_{18} = 0.12$   
 $\log(S_{18}/S_{19}) = 0.20$   
 $\log(S_{19}/S_{20}) = 0.33$

$\log(M_*/M_\odot) = 9.81$   
 $\log(M_{\text{H I}}/M_\odot) = 9.80$   
 $i = 47^\circ$

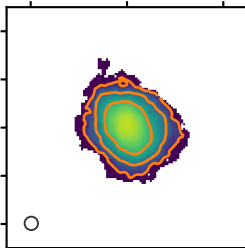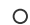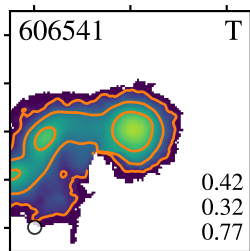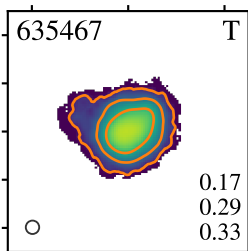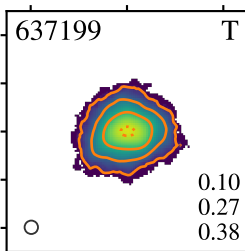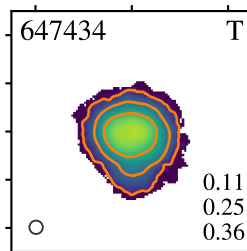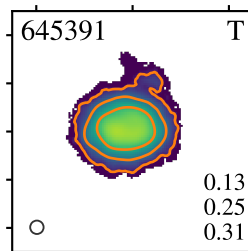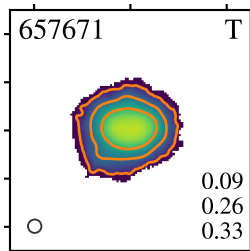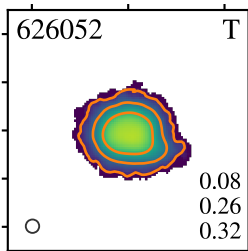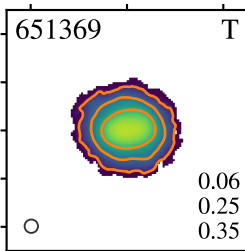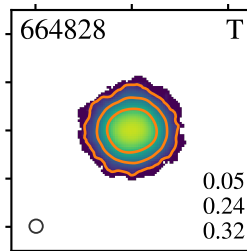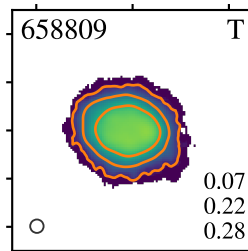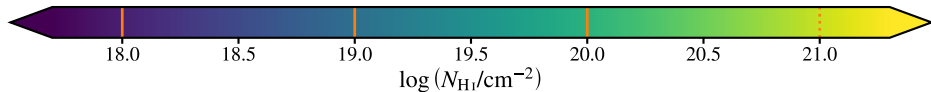

# NGC 660

$I_{18} = 0.19$   
 $\log(S_{18}/S_{19}) = 0.27$   
 $\log(S_{19}/S_{20}) = 0.39$

$\log(M_*/M_\odot) = 9.79$   
 $\log(M_{\text{H I}}/M_\odot) = 9.51$   
 $i = 74^\circ$

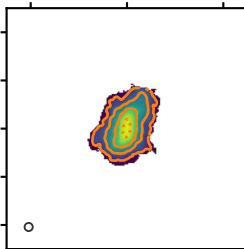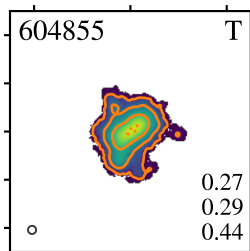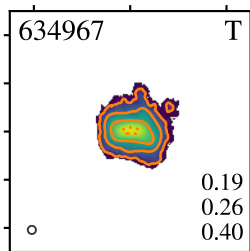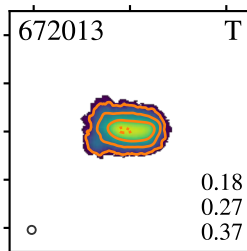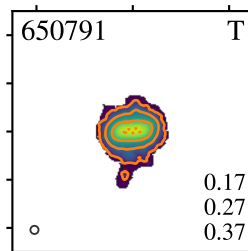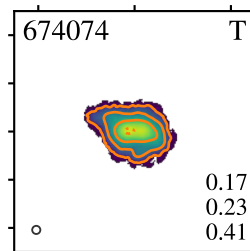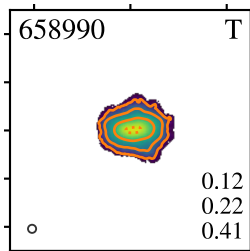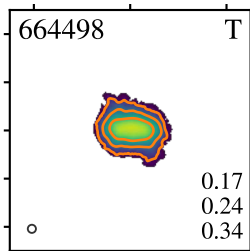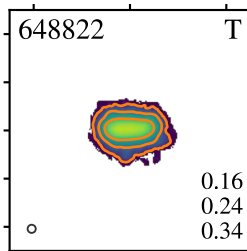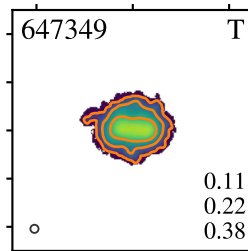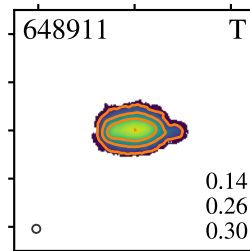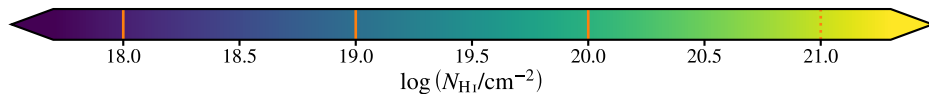

# NGC 925

$I_{18} = 0.11$   
 $\log(S_{18}/S_{19}) = 0.21$   
 $\log(S_{19}/S_{20}) = 0.37$

$\log(M_*/M_\odot) = 9.75$   
 $\log(M_{\text{H I}}/M_\odot) = 9.79$   
 $i = 66^\circ$

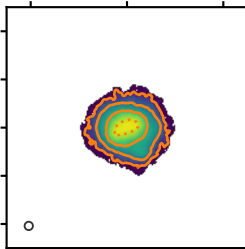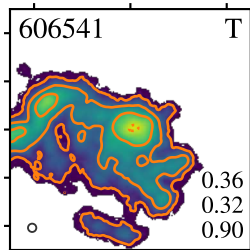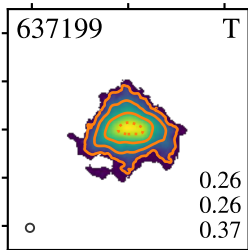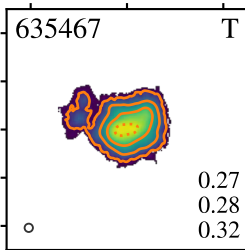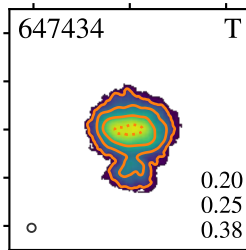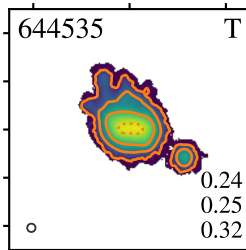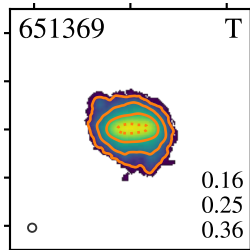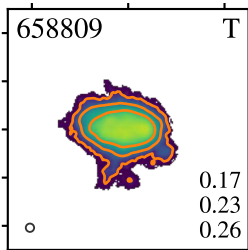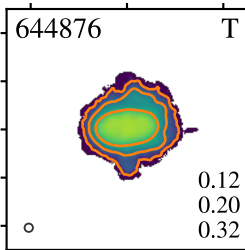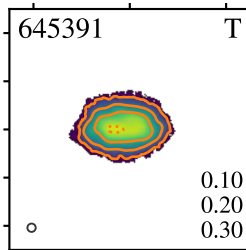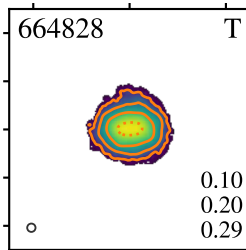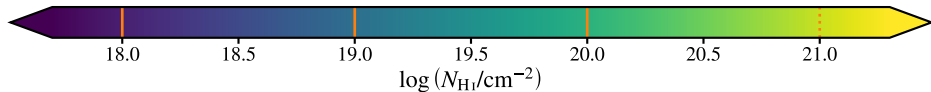

NGC 4490

$I_{18} = 0.20$   
 $\log(S_{18}/S_{19}) = 0.23$   
 $\log(S_{19}/S_{20}) = 0.62$

$\log(M_*/M_\odot) = 9.73$   
 $\log(M_{\text{H I}}/M_\odot) = 9.88$   
 $i = 63^\circ$

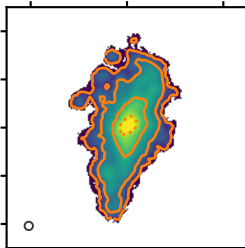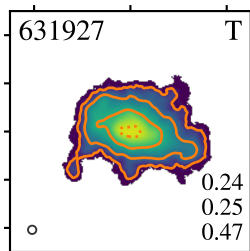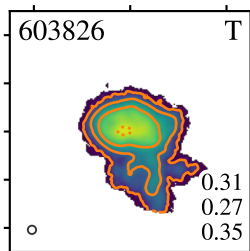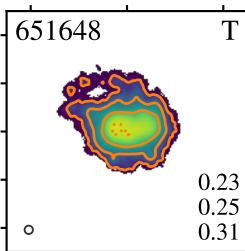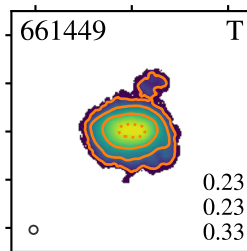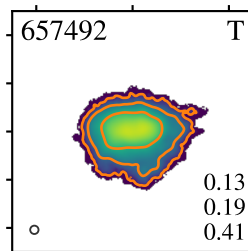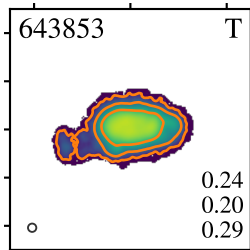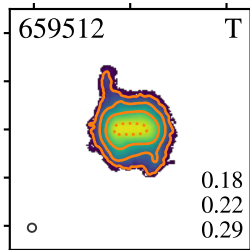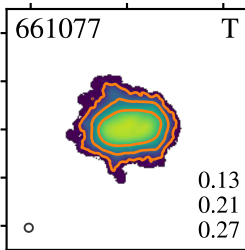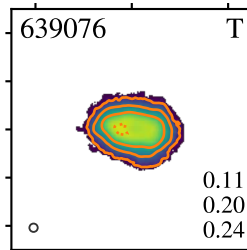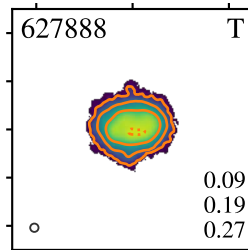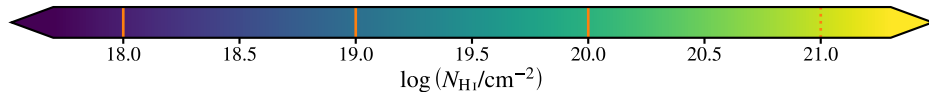

# NGC 3432

$I_{18} = 0.15$   
 $\log(S_{18}/S_{19}) = 0.23$   
 $\log(S_{19}/S_{20}) = 0.40$

$\log(M_*/M_\odot) = 9.66$   
 $\log(M_{\text{H I}}/M_\odot) = 9.84$   
 $i = 76^\circ$

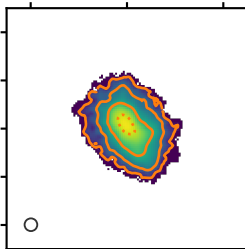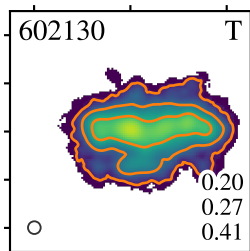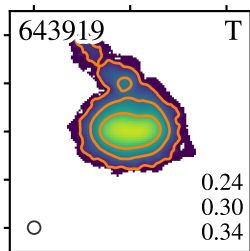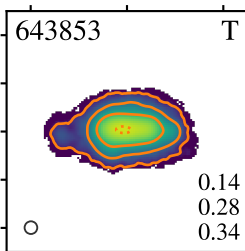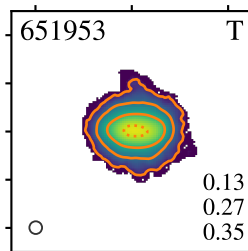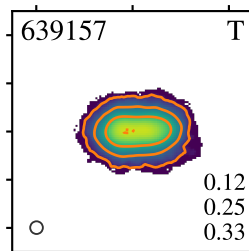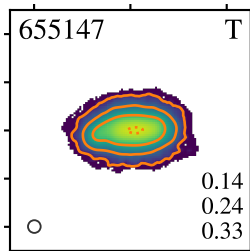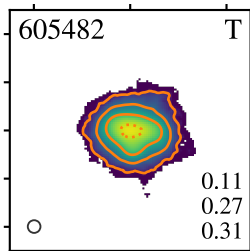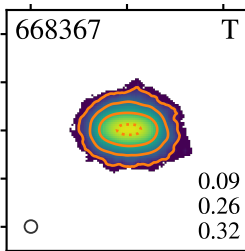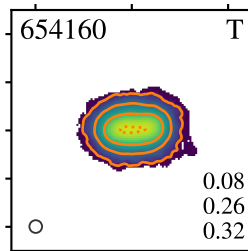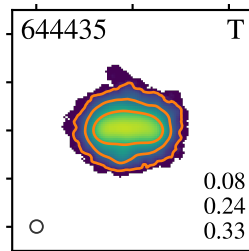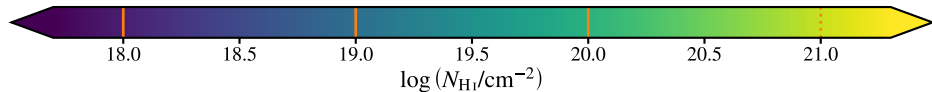

Supplement: Supplementary file 1 [file atlas.pdf]
